# Supplementary material for: To what extent can we analyze Kotlin programs using existing Java taint analysis tools? (Extended Version)
Source: arXiv:2207.09379 source file (2022-07-29)
Supplement: Supplementary file 1 [file additional.tex]

\section{Additional found problems}
\label{sec:additional}

Explain the remaining problems we found in short. May be give two tables which dont have any problem and another table for the features associated with some problems (Like in my thesis).
